# Supplementary material for: Conformal Prediction: A Theoretical Note and Benchmarking Transductive Node Classification in Graphs
Source: arXiv:2409.18332 source file (2025-05-19)
Supplement: Supplementary file 1 [file aps_appendix.tex]

Here, we prove Theorem \ref{them:APS:efficiency}, to provide a framework that can be used to compare the efficiency of two non-conformity scores. 

Let $A(\vx, y) $ and $\tilde{A}(\vx, y)$ be non-conformity scores. Let
\[
    \hat{q}_{A} = \text{Quantile}\left(\frac{\ceil{(n+1)(1-\alpha)}}{n}; \{A(\vx_i, y_i)\}_{i=1}^{n}\right)
\]
and
\[
    \hat{q}_{\Tilde{A}} = \text{Quantile}\left(\frac{\ceil{(n+1)(1-\alpha)}}{n}; \{\Tilde{A}(\vx_i, y_i)\}_{i=1}^{n}\right)
\]
Define $A_i(y) := A(\vx_i, y)$ and $\Tilde{A}_i(y) := \Tilde{A}(\vx_i, y)$.
From the definition of the prediction sets and non-conformity scores, we have 
\[
    C_A(\vx_{n+1}) = \{y \in \gY: A_{n+1}(y) \leq \hat{q}_{A}\}
\] and 
\[
    C_{\Tilde{A}}(\vx_{n+1}) = \{y \in \gY: \Tilde{A}_{n+1}(y) \leq \hat{q}_{\Tilde{A}}\}
\] 
denote the prediction sets corresponding to the two score functions (e.g. APS with and without randomization).
Define $C_{A}^{i} = C_{A}(\vx_{i})$. 
Let $y'_i \in \{1, 2, \dots, K\} \setminus \{y_i\}$ be any incorrect class label for each $\vx_i$.
Define 
\[
    \alpha_c^A \in [0, 1], \hat{q}_A = \text{Quantile}\left( \frac{\ceil{(n+1)(1 - \alpha_c^A)}}{n}; \{A(\vx_i, y'_i)\}_{i=1}^n \right)
\]
\[
    \alpha_c^{\Tilde{A}} \in [0, 1], \hat{q}_{\Tilde{A}} = \text{Quantile}\left( \frac{\ceil{(n+1)(1 - \alpha_c^{\Tilde{A}})}}{n}; \{\Tilde{A}(\vx_i, y'_i)\}_{i=1}^n \right)
\]    
as the thresholds for which the corresponding quantile of the scores for the correct classes $A_i(y_i)$ and $\Tilde{A}_i(y_i)$ achieve $1-\alpha$ coverage.

Then from the exchangeability of $A(\vx_i, y'_i)$
\[
    1 - \alpha_c^A \leq \Pr[y'_{n+1} \in C_{A}^{n+1}] \leq 1 - \alpha_c^A + \frac{1}{n+1}
\]
and similarly, from the exchangeability of $\Tilde{A}(\vx_i, y'_i)$
\[
    1 - \alpha_c^{\Tilde{A}} \leq \Pr[y'_{n+1} \in C_{\Tilde{A}}^{n+1}] \leq 1 - \alpha_c^{\Tilde{A}} + \frac{1}{n+1}
\]

With this setup, we restate Theorem~\ref{them:APS:efficiency} and prove it below.
\apsEff*

\begin{proof}
Consider the case with only two potential class labels $K = \{1, 2\}$. 

Then, we have
\begin{align*}
    \E\left[|C_{A}^{n+1}|\right] &= \E\left[\sum\limits_{i=1, 2}\1[i \in C_{A}^{n+1}]\right] \\
                                 &= \E\left[\1[y_{n+1} \in C_{A}^{n+1}]\right] + \E\left[\1[y'_{n+1} \in C_{A}^{n+1}]\right]  & \text{linearity}\\
                                 &= \Pr[y_{n+1} \in C_{A}^{n+1}] + \Pr[y'_{n+1} \in C_{A}^{n+1}] & \text{$\E[\1[A]] = \Pr[A]$}\\
                                 &\leq 1 - \alpha + 1 - \alpha_c^A + \frac{2}{n+1} & \text{(Exchangeability, Theorem~\ref{thm:CP:coverage})} 
\end{align*}
From a similar argument, we can show that 
\[
    \E\left[|C_{\Tilde{A}}^{n+1}|\right] \geq 1 - \alpha + 1 - \alpha_c^{\Tilde{A}}
\]
Thus, 
\begin{align}
    \E\left[|C_{\Tilde{A}}^{n+1}| - |C_{A}^{n+1}|\right] &\geq 1 - \alpha + 1 - \alpha_c^{\Tilde{A}} - \left(1 - \alpha + 1 - \alpha_c^A + \frac{2}{n+1} \right)\\
    &= \alpha_c^A - \alpha_c^{\Tilde{A}} - \frac{2}{n+1}
\end{align}
which is equivalent to our assumption, and this completes the proof.

For $K$ classes, 
\begin{align*}
    \E\brackets{\abs{C_{A}^{n+1}}} &= \Pr[y_i \in C_{A}^{n+1}] + \sum\limits_{y'_i} \Pr[y'_i \in C_{A}^{n+1}] \\
     &= \Pr[y_i \in C_{A}^{n+1}] + (K-1)\Pr[y'_i \in C_{A}^{n+1}] \\
\end{align*}
Thus, 
\begin{align*}
    \E\brackets{\abs{C_{A}^{n+1}}}&\leq 1 - \alpha + \frac{1}{n+1} + (K-1)\left(1 - \alpha_c^A + \frac{1}{n+1}\right) \\
     &= 1 - \alpha + (K-1)\left( 1 - \alpha_c^A\right) + \frac{K}{n+1}
\end{align*}
and 
\[
    \E\brackets{\abs{C_{A}^{n+1}}} \geq 1 - \alpha + (K-1)\left(1 - \alpha_c^A\right)
\]
similar bounds can be derived for $\E\brackets{\abs{C_{\Tilde{A}}^{n+1}}}$.
Thus, 
\begin{align*}
    \E\left[|C_{\Tilde{A}}^{n+1}| - |C_{A}^{n+1}|\right] &\geq (K-1)\left(\alpha_c^A - \alpha_c^{\Tilde{A}}\right) - \frac{K}{n+1} \\
    &\geq (K-1) \left(\alpha_c^A - \alpha_c^{\Tilde{A}} - \frac{K}{(K-1)(n+1)}\right)\\
    & >  (K-1)\left(\alpha_c^A - \alpha_c^{\Tilde{A}} - \frac{2}{n+1}\right) \geq 0 & \text{Since } \alpha_c^A - \alpha_c^{\Tilde{A}} \geq \frac{2}{n+1}
\end{align*}
Which completes the proof in the general case.

\end{proof}
